# Supplementary material for: Deep Reinforcement Learning for Complex Manipulation Tasks with Sparse Feedback
Source: arXiv:2001.03877 source file (2020-01-12)
Supplement: Supplementary file 1 [file AppendixTemplate.tex]

% Appendix Template

\chapter{Appendix Title Here} % Main appendix title

\label{AppendixX} % Change X to a consecutive letter; for referencing this appendix elsewhere, use \ref{AppendixX}

Write your Appendix content here.
